# Supplementary material for: DETR3D: 3D Object Detection from Multi-view Images via 3D-to-2D Queries
Source: arXiv:2110.06922 source file (2021-10-13)
Supplement: Supplementary file 1 [file supplement.tex]

\section*{Supplementary Material}
\subsection*{Comparison to FCOS3D without global NMS.}
We also compare our MVOD method to FCOS3D without global NMS. We test in both settings: benchmarking using all data and using ground-truth bounding boxes only in the overlap regions. As shown in Table~\ref{table:global-nms}, our model outperforms FCOS3D without global NMS. This suggests that FCOS3D is very reliant on global NMS, with a significant drop in performance when it is disabled, while our method completely eliminates the need for it. In addition, we also remove the per-image NMS in FCOS3D and the model fails. So we ignore the results in this table. 
%without global NMS, the performance of FCOS3D drops significantly while our model is robust to NMS. 

\begin{table}[t] 
\begin{center}
\caption{Comparisons to FCOS3D without global NMS. \label{table:global-nms}}
\resizebox{\linewidth}{!}{
\begin{tabular}{c|c|c|c|c|c|c|c|c|c}
\toprule
\hline
Method & NDS $\uparrow$ & mAP $\uparrow$ & mATE $\downarrow$ & mASE $\downarrow$ & mAOE $\downarrow$ & mAVE $\downarrow$ & mAAE $\downarrow$ & global NMS  & overlap region only \\
\hline
FCOS3D $\ddag$ & 0.273 & 0.133 & 0.890 & 0.274 & 0.593 & 1.093 & 0.176 & - & 
\checkmark \\
\hline
FCOS3D & 0.317 & 0.213 & 0.841 & 0.276 & 0.604 & 1.122 & 0.173 &  \checkmark & \checkmark \\
\hline 
\name (Ours)  &  0.356 & 0.231 & 0.825 & 0.280 & 0.400 & 0.863 & 0.223 & - & \checkmark \\
\hline
FCOS3D $\ddag$ & 0.336 & 0.234 & 0.830 & 0.268 & 0.558 & 1.361 & 0.153 & - & - \\
\hline
FCOS3D $\ddag$ & 0.373 & 0.299 & 0.785 & 0.268 & 0.557 & 1.396 & 0.154 & \checkmark & - \\
\hline
\name (Ours)  &  0.374 & 0.303 & 0.860 & 0.278 & 0.437 & 0.967 & 0.235 & - & - \\
\hline
\bottomrule
\end{tabular}
}
\end{center}
\end{table}

\subsection*{Time complexity.}
We compare the time complexity of FCOS3D with and without global NMS to that of our proposed MVOD model. Table~\ref{table:time-complexity} shows that MVOD is more efficient at inference time thanks to its NMS-free design. We also provide the performance when the NMS is not used in the FCOS3D. The per-image NMS contributes to a large portion of the overhead, which is not required by our model. 
We also note that further improvements in efficiency can be achieved by implementing more GPU-friendly feature sampling in our model. These frame rates were measured on a single Nvidia RTX 3090.

\begin{table}[t] 
\begin{center}
\caption{Time complexity.\label{table:time-complexity}}
 \vspace{-1.5em}
\resizebox{\linewidth}{!}{
\begin{tabular}{c|c|c|c|c}
\toprule
\hline
Models & FCOS3D & FCOS3D (w/o global NMS) & FCOS3D (w/o global NMS, w/o per-image NMS) & MVOD (ours)  \\
\hline
FPS & 1.1 & 1.2 & 3.3 & 3.1 \\
\hline
\bottomrule
\end{tabular}
}
\end{center}
\end{table}
